# Supplementary material for: Multimodal Emergent Fake News Detection via Meta Neural Process Networks
Source: arXiv:2106.13711 source file (2021-06-22)
Supplement: Supplementary file 1 [file 7_appendix.tex]

\section{K-shots}

\noindent\textbf{Effect of varying the number of few-shots K.} We show the performance changes with respect to varying number of few-shots K $\{5, 10, 20, 100\}$ on Wikiann (en), MIT movie, MIT Restaurant, CoNLL2003 (En), Multilingual CoNLL and Multilingual Wikiann  in Table 9-13. Since the maximum number of  labeled examples for some slots in Email dataset is around 10, we only show 5 and 10 shots for Email dataset in Table 8. 
\begin{table}[!htb]
\centering
\caption{Email Dataset.} 
\resizebox{0.7\linewidth}{!}{
\begin{tabular}{c|cc}
\toprule

\multirow{2}{*}{Method} &
\multicolumn{2}{c}{Shots}\\

\cline{2-3}
 & 
5  & 10 \\
\midrule
\midrule
\multicolumn{3}{l}{\textbf{Full-supervision}}\\
BERT & \multicolumn{2}{c}{0.9444}  \\
\midrule
\multicolumn{3}{l}{\textbf{Few-shot Supervision}}\\
BERT & 0.8211 & 0.8785 \\
\midrule
\multicolumn{3}{l}{\textbf{Few-shot Supervision} + \textbf{unlabeled data}}\\
CVT & 67.44& 78.24 \\
SeqVAT & 64.67 & 72.65\\

Mean Teacher & 84.10&89.53  \\
VAT &  83.24& 89.71\\
Classic ST & 86.88 & 90.70  \\

BOND & 84.92 & 89.75\\
\midrule
MetaST & 89.21 &92.18\\

\bottomrule
\end{tabular}
}
\end{table}

\begin{table}[!htb]
\centering
\small

\resizebox{0.9\linewidth}{!}{
\begin{tabular}{c|cccc}
\toprule

\multirow{2}{*}{Method} &
\multicolumn{4}{c}{Shots (3 Slot Types)}\\

\cline{2-5}
 & 
5  & 10 & 20 & 100\\
\midrule
\midrule
\multicolumn{3}{l}{\textbf{Full-supervision}}\\
BERT &  \multicolumn{4}{c}{84.04} \\
\midrule
\multicolumn{3}{l}{\textbf{Few-shot Supervision}}\\
BERT  & 37.01 & 45.61 & 54.53 & 67.87\\
\midrule
\multicolumn{3}{l}{\textbf{Few-shot Supervision} + \textbf{unlabeled data}}\\
CVT &16.05 & 27.89 & 46.42&66.36\\
SeqVAT & 21.11 & 35.16&42.26&62.37\\
Mean Teacher & 30.92 & 41.43 & 50.61 & 67.16\\
VAT & 24.72 & 38.81 & 50.15 & 66.31\\
Classic ST & 32.72 & 46.15 & 54.41 & 68.64\\
BOND & 34.22 & 48.73 & 52.45 & 68.89 \\
\midrule
MetaST &55.04& 56.61 & 60.38 & 73.20\\

\bottomrule
\end{tabular}
}
\caption{Wikiann (En) Dataset.} % The $0.05\%$ and $5\%$ of unlabeled data are similar with CoNLL03 and SNIPS 10 labeled data sizes respectively.
\end{table}

\begin{table}[!htb]
\centering
\resizebox{0.9\linewidth}{!}{
\begin{tabular}{c|cccc}
\toprule

\multirow{2}{*}{Method} &
\multicolumn{4}{c}{Shots (12 Slot  Types)}\\

\cline{2-5}
 & 
5  & 10 & 20 & 100\\
\midrule
\midrule
\multicolumn{3}{l}{\textbf{Full-supervision}}\\
BERT  & \multicolumn{4}{c}{87.87} \\
\midrule
\multicolumn{3}{l}{\textbf{Few-shot Supervision}}\\
BERT & 62.80 & 69.50 & 75.81 & 82.49\\
\midrule
\multicolumn{3}{l}{\textbf{Few-shot Supervision} + \textbf{unlabeled data}}\\
CVT & 57.48 &  62.73&70.20&81.82 \\
SeqVAT & 60.94 & 67.10 & 74.15 & 82.73\\
Mean Teacher & 58.92 & 67.62 & 75.24 & 82.20\\
VAT & 60.75 & 70.17 & 75.41 & 82.39\\

Classic ST & 63.39 & 71.88  & 76.58 & 83.06\\
BOND & 62.50 & 70.91  & 75.52 & 82.65\\
\midrule
MetaST & 72.57 & 77.67 &80.33 & 84.35 \\
\bottomrule
\end{tabular}
}\caption{MIT Movie Dataset.} 
\end{table}

\begin{table}[!htb]
\centering

\resizebox{0.9\linewidth}{!}{
\begin{tabular}{c|cccc}
\toprule

\multirow{2}{*}{Method} &
\multicolumn{4}{c}{Shots (8 Slot Types)}\\

\cline{2-5}
 & 
5  & 10 & 20 & 100\\
\midrule
\midrule
\multicolumn{3}{l}{\textbf{Full-supervision}}\\
BERT & \multicolumn{4}{c}{78.95}\\
\midrule
\multicolumn{3}{l}{\textbf{Few-shot Supervision}}\\
BERT & 41.39 & 54.06 & 60.12 & 72.24\\
\midrule
\multicolumn{3}{l}{\textbf{Few-shot Supervision} + \textbf{unlabeled data}}\\
CVT &33.74 &42.57 & 51.33 &70.84\\
SeqVAT & 41.94 & 51.55 & 56.15 & 71.39\\
Mean Teacher & 40.37 & 51.75 & 57.34 & 72.40\\
VAT & 41.29 & 53.34 & 59.68 & 72.65 \\
Classic ST & 44.35 & 56.80& 60.28 & 73.13 \\
BOND & 43.01 &  55.78 &  59.96 & 73.60 \\
\midrule
MetaST &53.02 & 63.83& 67.86 &  75.25\\

\bottomrule
\end{tabular}
}
\caption{MIT Restaurant Dataset.} % 
\end{table}

\begin{table}[!htb]
\centering
\resizebox{0.9\linewidth}{!}{
\begin{tabular}{c|cccc}
\toprule
\multirow{2}{*}{Method} &
\multicolumn{4}{c}{Shots (4 Slot Types)}\\
\cline{2-5}
 & 
5  & 10 & 20 & 100\\
\midrule
\midrule
\multicolumn{3}{l}{\textbf{Full-supervision}}\\
BERT & \multicolumn{4}{c}{92.40}\\
\midrule
\multicolumn{3}{l}{\textbf{Few-shot Supervision}}\\
BERT  & 63.87 & 71.15 & 73.57 &84.36\\
\midrule
\multicolumn{3}{l}{\textbf{Few-shot Supervision} + \textbf{unlabeled data}}\\
CVT & 51.15 &54.31 &66.11&81.99\\
SeqVAT & 58.02 &67.21&74.15&82.20\\
Mean Teacher &59.04 &68.67 &72.62&84.17\\
VAT & 57.03 & 65.03&72.69&84.43\\
Classic ST & 64.04 & 70.99 &74.65&84.93 \\
BOND &62.52  & 69.56 &74.19&83.87\\
\midrule
MetaST &71.49&76.65 & 78.54 & 85.77 \\

\bottomrule
\end{tabular}
}\caption{CoNLL2003 (EN)} 
\end{table}

% We can observe that the performance of each model increases as number of shots increases. Our method brings consistent improvement across different shots and different datasts. 

\begin{table}[!hbt]
\centering
\resizebox{0.9\linewidth}{!}{
\begin{tabular}{c|cccc}
\toprule

\multirow{2}{*}{Method} &
\multicolumn{4}{c}{Shots (3 Slot Types $\times$ 41 languages)}\\

\cline{2-5}
 & 
5  & 10 & 20 & 100\\
\midrule
\midrule
\multicolumn{3}{l}{\textbf{Full-supervision}}\\
BERT &  \multicolumn{4}{c}{87.17 }\\
\midrule
\multicolumn{3}{l}{\textbf{Few-shot Supervision}}\\
BERT  & 77.68 & 79.67 & 82.33 & 85.70 \\
\midrule
\multicolumn{3}{l}{\textbf{Few-shot Supervision} + \textbf{unlabeled data}}\\
Mean Teacher & 77.09 & 80.23 & 82.19 & 85.34\\
VAT & 74.71 & 78.82 & 82.60 & 85.82\\
Classic ST & 76.73  & 80.24 & 82.39 & 86.08\\
BOND & 78.81 & 79.57 & 82.19&86.14 \\
\midrule
MetaST &79.10& 81.61 & 83.14 & 85.57\\

\bottomrule
\end{tabular}
}\caption{Multilingual Wikiann} 
\end{table}

\begin{table}[!hbt]
\centering
\resizebox{0.9\linewidth}{!}{
\begin{tabular}{c|cccc}
\toprule

\multirow{2}{*}{Method} &
\multicolumn{4}{c}{Shots (4 Slot Types)}\\

\cline{2-5}
 & 
5  & 10 & 20 & 100\\
\midrule
\midrule
\multicolumn{3}{l}{\textbf{Full-supervision}}\\
BERT & \multicolumn{4}{c}{87.67} \\
\midrule
\multicolumn{3}{l}{\textbf{Few-shot Supervision}}\\
BERT  & 64.80 & 70.77 & 73.89 & 80.61 \\
\midrule
\multicolumn{3}{l}{\textbf{Few-shot Supervision} + \textbf{unlabeled data}}\\
Mean Teacher & 64.55 &68.34&73.87&79.21\\
VAT &64.97 & 67.63 & 74.26 & 80.70  \\
Classic ST &67.95 &  72.69&73.79&81.82\\
BOND & 69.42 & 72.79 & 76.02 & 80.62  \\
\midrule
MetaST &73.34 &  76.65 & 77.01 & 82.11\\

\bottomrule
\end{tabular}
}
\caption{Multilingual CoNLL03.} % 
\end{table}

\section{Implementations and Hyper-parameter}

We do not perform any hyper-parameter tuning for different datasets. The training batch size for each dataset is 16. The maximum sequence length varies due to data characteristics. For  and are as shown in Table~\ref{tab:uda}. The hyper-parameters are as shown in Table~\ref{tab:hyper}.

Also, we retain parameters from original BERT implementation from \url{https://github.com/huggingface/transformers}.
 
We implement SeqVAT based on \url{https://github.com/jiesutd/NCRFpp} and implement CVT following \url{https://github.com/tensorflow/models/tree/master/research/cvt_text}.

\begin{table}[!htb]
\small
\centering
\resizebox{\linewidth}{!}{
    \begin{tabular}{lccccl}
    \toprule
    Dataset & Sequence  Length & Batch Size & Labeled data sample size $|\mathcal{B}|$& Unlabeled Batch Size & BERT Encoder\\
    \midrule
    SNIPS & 64  & 32 &32&BERT-base-uncased \\
    Email     & 64  & 16 &32& 32 &BERT-base-cased\\
    Movie & 64   & 32 &32 & BERT-base-uncased \\
    Restaurant &  64   & 16 & 32 &BERT-base-uncased \\
    CoNLL03 (EN) & 128  & 8 & 32 &BERT-base-cased \\
    Wikiann (EN) & 128  & 8 &32 &BERT-base-cased\\
    CoNLL03 (multilingual) & 128  & 32&32 & BERT-multilingual-base-cased\\
    Wikiann (multilingaul)&128  &32 &32 & BERT-multilingual-base-cased\\
    \bottomrule
    \end{tabular}
}
    \caption{Batch size, sequence length and BERT encoder choices across datasets}
    \label{tab:hyper}
\end{table}

\begin{table}[hbt]
\small
\centering
\resizebox{\columnwidth}{!}{
    \begin{tabular}{lr}
    \toprule
    BERT attention dropout & 0.3 \\
    BERT hidden dropout & 0.3 \\
    Latest Iteration R in labeled data acquisition & 5 \\
    BERT output hidden size $h$ & 768 \\\midrule
    Steps for fine-tuning teacher model on labeled data & 2000 \\
    Steps T for self-training model on unlabeled data & 3000\\
    Mini-batch S & 5 \\
    Re-initialize Student & Y\\
    Pseudo-label Type & Hard \\
    Warmup steps & 20 \\
    learning rate $\alpha$ & $5e^{-5}$ \\
    Weight\_decay & $5e^{-6}$ \\
    \bottomrule
    \end{tabular}
}
    \caption{Hyper-parameters.}
    \label{tab:uda}
\end{table}
